# Supplementary material for: Learning to Communicate to Solve Riddles with Deep Distributed Recurrent Q-Networks
Source: arXiv:1602.02672 source file (2016-02-08)
Supplement: Supplementary file 1 [file 0_supplementary.tex]

\section{Network Architecture}

\begin{figure}[h]
    \centering
    \begin{subfigure}[t]{0.526\textwidth} %0.585
	    \centering
	    \includegraphics[width=1\linewidth]{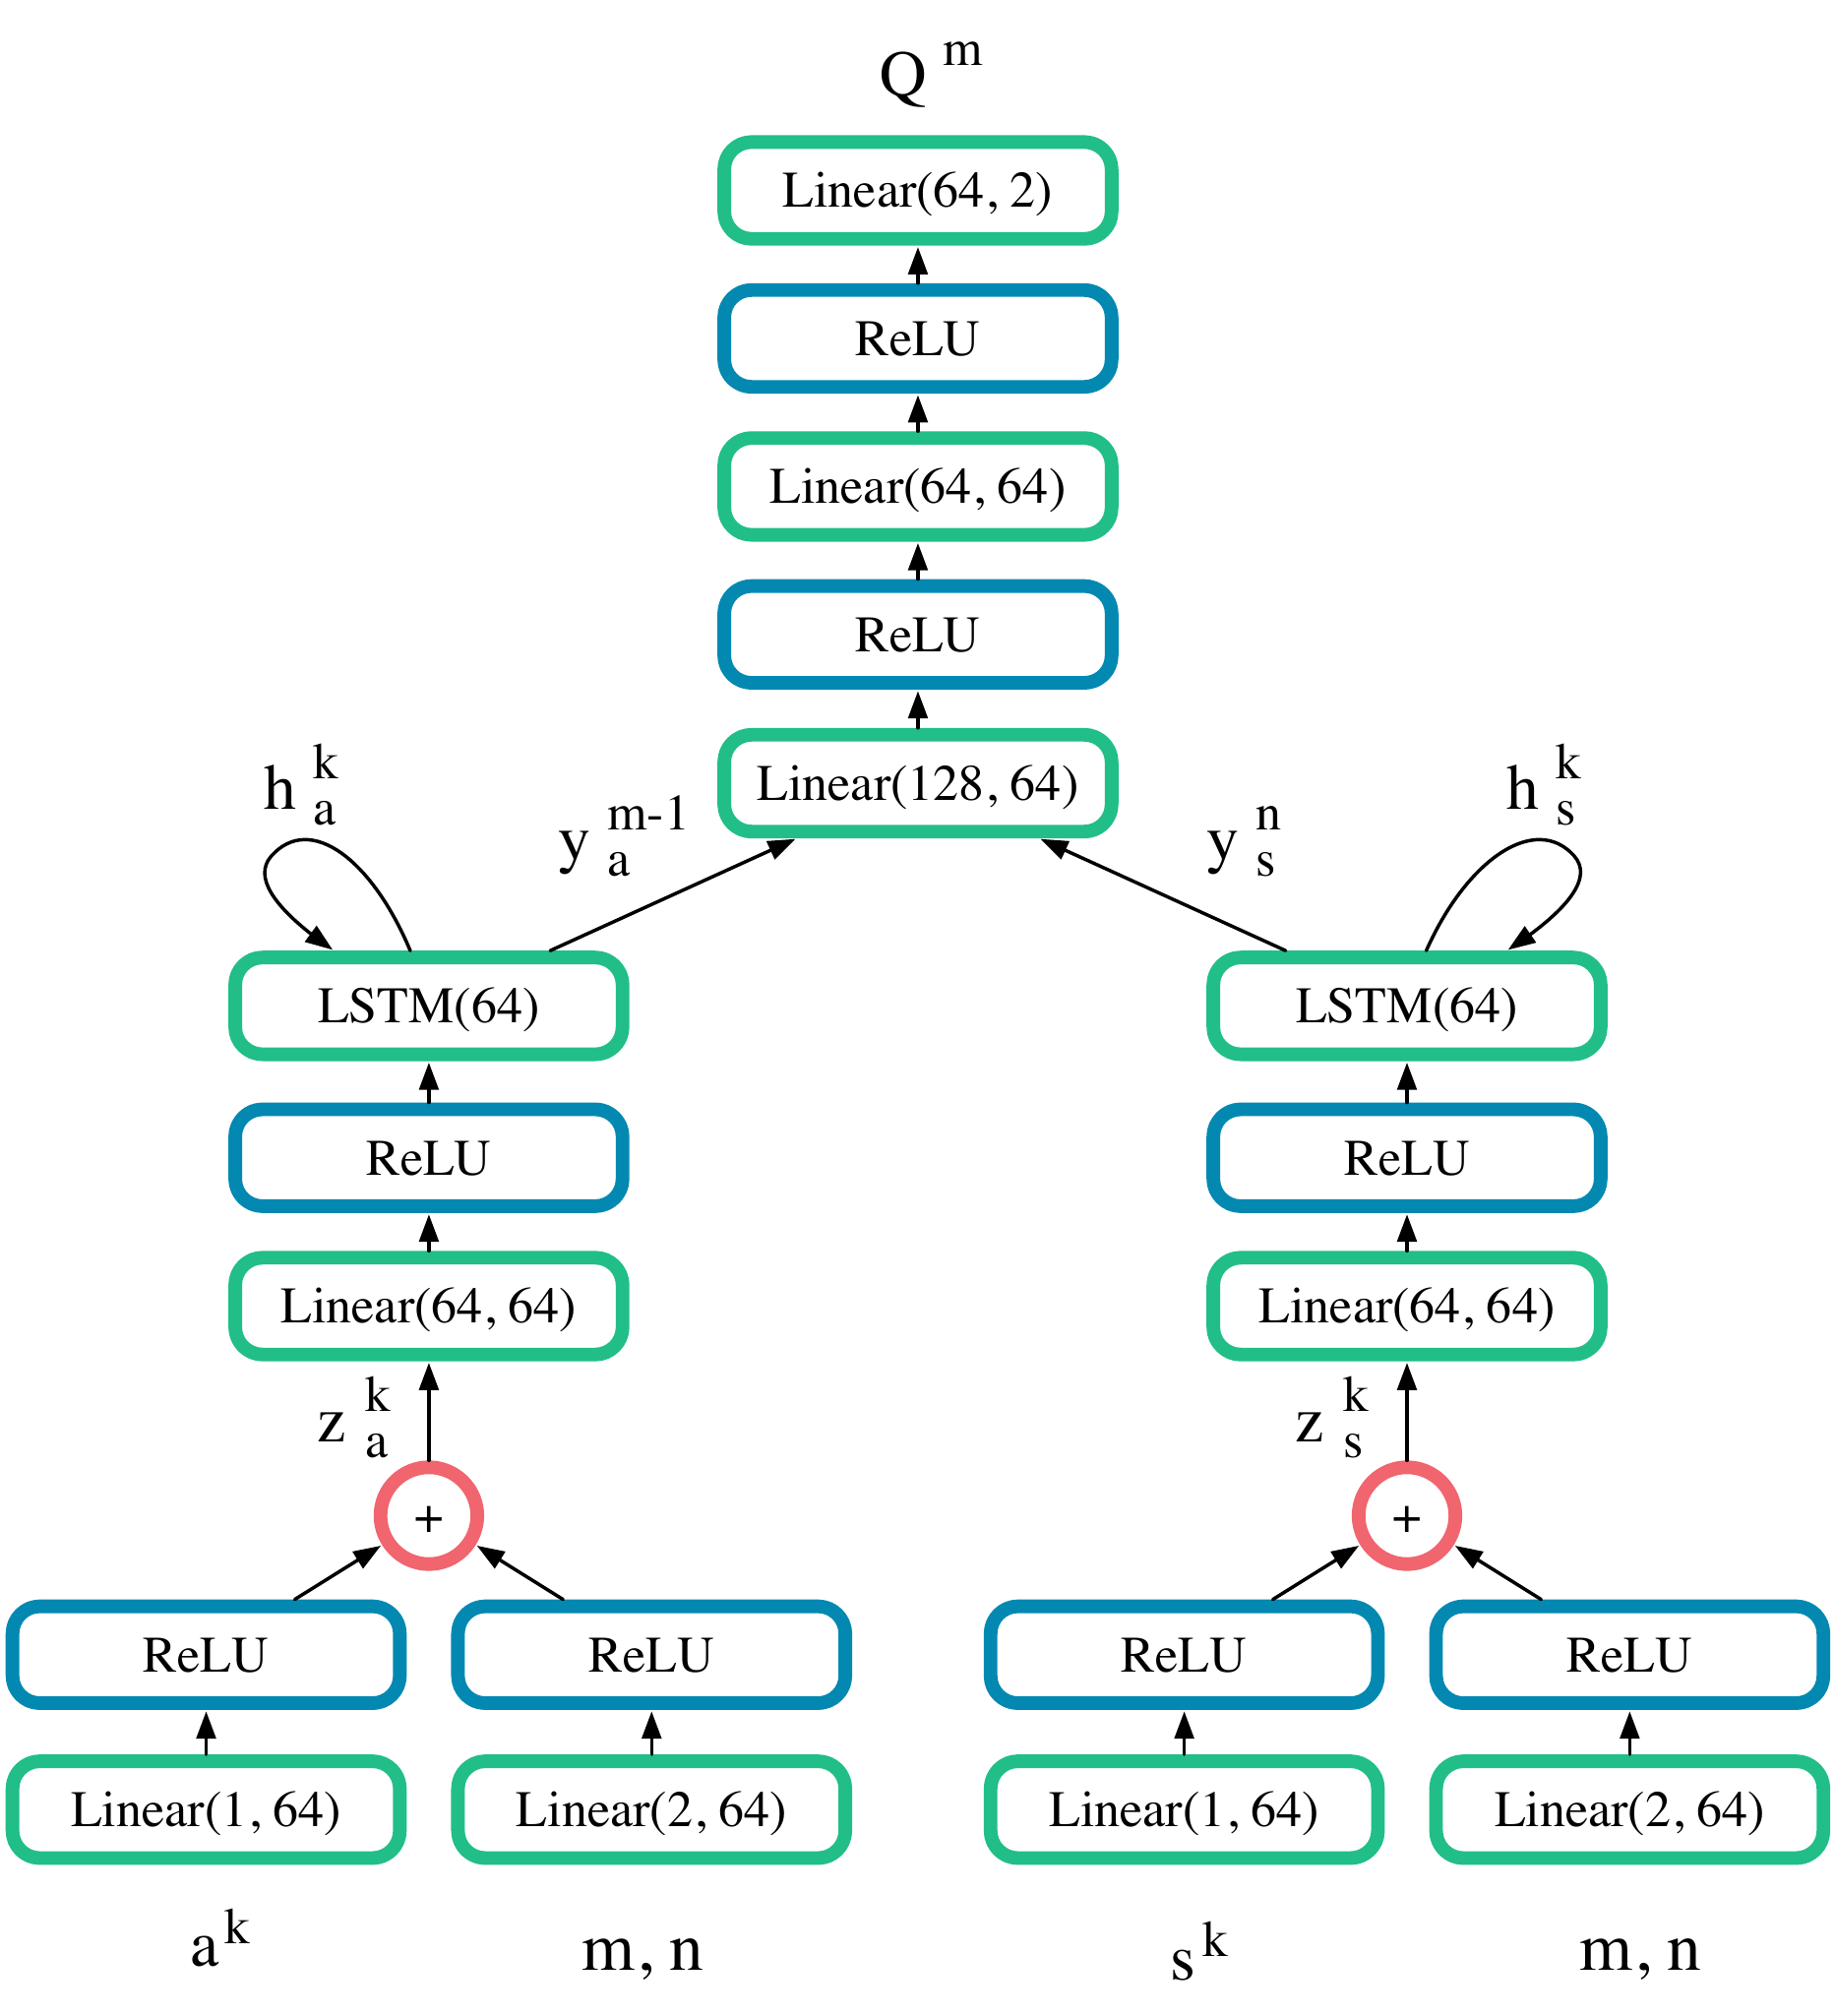}
	    \caption{\emph{Hats:} Each agent $m$ sequentially observes the answers, $a^k$, from all proceeding agents $k$, $k<m$, and the colour of the hats, $s^k$ in front of him, $k > m$.  At each step both $a$ and $s$ are passed through  fully connected layers and then fed into two RNNs for processing, $\phi_\text{R\_a}$ and $\phi_\text{R\_s}$,  together with the agent index $m$ and the total number of agents $n$. The final output of these RNNs are used to compute the Q-value, $Q^m_t$, from which the action $a^m_t$ is chosen.}
	    \label{fig:hats_arch}
    \end{subfigure}%
    \hspace{0.05\textwidth}
    \begin{subfigure}[t]{0.373\textwidth} %0.415
	    \centering
	    \includegraphics[width=1\linewidth]{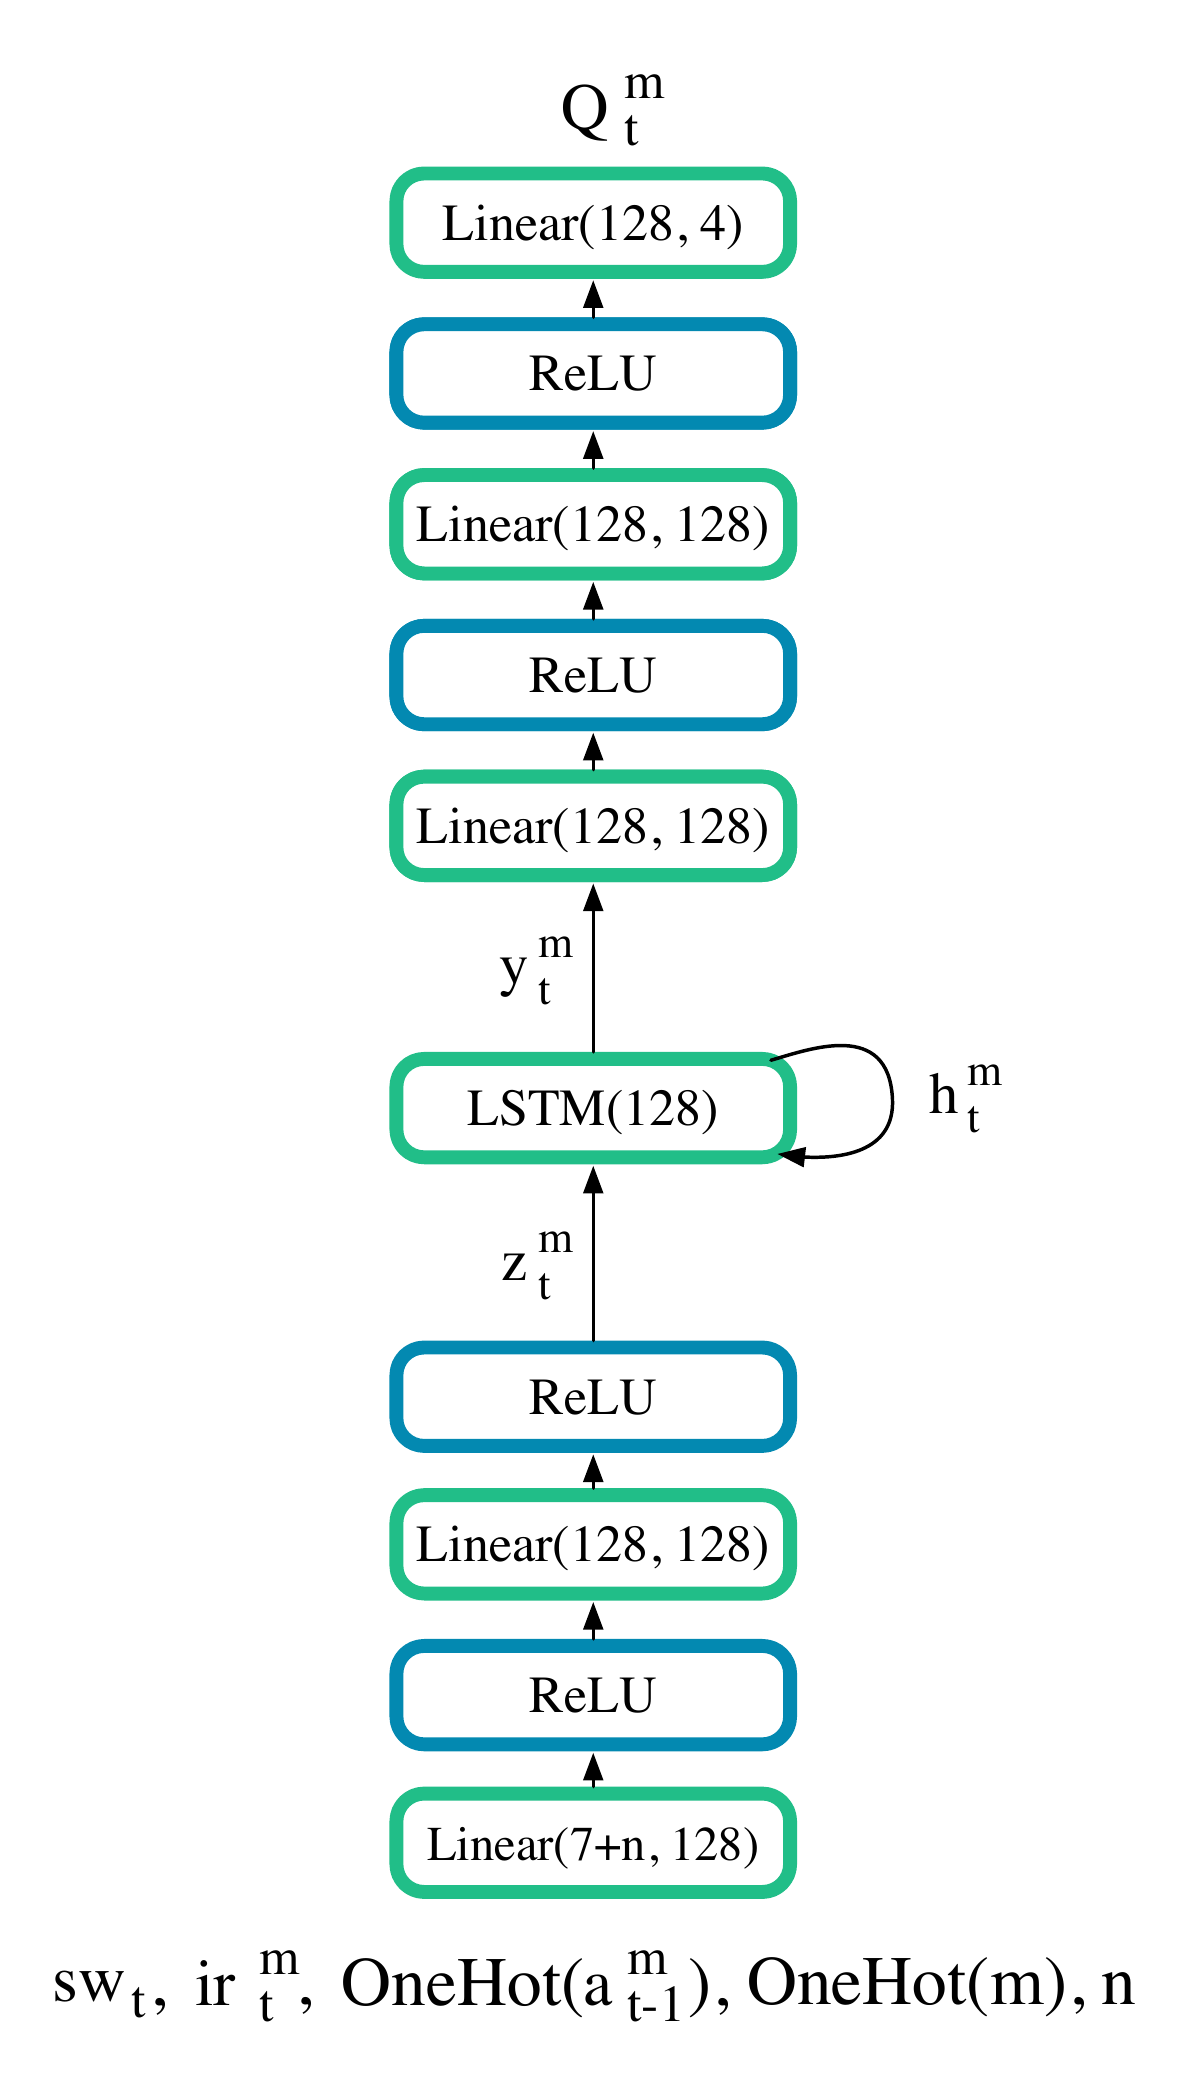}
	    \caption{\emph{Switch:} Agent $m$ receives as input: $sw_t$, his last action, $a^m_{t-1}$, his ID, $m$,  the $\#$ of agents, $n$, and the room he is in, $lr^m_t$. The inputs are fed through a transformation $\phi_{in}$ and then passed to a RNN $\phi_R$. The output is fed through $\phi_{out}$ and  used to compute the Q-values for the four actions, $\mathcal{A}$: ``On'', ``Off'', ``Tell'' and ``none''. }
	    \label{fig:switch_arch}
    \end{subfigure}
    \caption{DDRQN architecture for the Hats and Switch riddles.}
\end{figure}

\newpage

\section{Strategy Visualisation}

\begin{table}[h]
\caption{\emph{Hats}: We sampled 10k episodes of $n=4$ after training had converged. For a combination of day and  previous total number of visitors that have been to the interrogation room we show how often the active agent picks what action. It is evident that mostly the agents encode 2 visitors with the ``On'' positions and 3 visitors with the ``Off'' position.}
\label{table:hats-strategy}
\vskip 0.15in
\begin{center}
\begin{small}
\begin{sc}
\begin{tabular}{|r|c|r|r|r|}
\hline
\abovespace\belowspace
Day & \multicell{\# prisoners \\ that have \\ been in} & off & on & tell \\ 
\hline
\abovespace
1   & 1    & 10000 &      &    \\ \hline
\multirow{2}{*}{2}   & 1    &       & 2521 &    \\ 
    & 2    & 7479  &      &    \\ \hline
\multirow{3}{*}{3}   & 1    &       & 632  &    \\ 
    & 2    &       & 5574 &    \\
    & 3    & 3794  &      &    \\ \hline
\multirow{4}{*}{4}   & 1    &       & 164  &    \\ 
    & 2    & 468   & 2729 &    \\ 
    & 3    & 5681  &      &    \\ 
    & 4    &       &      & 958    \\ \hline
\multirow{4}{*}{5}   & 1    &       & 47   &    \\
    & 2    & 231   & 1526 &    \\
    & 3    & 5547  &      & 240    \\
    & 4    &       &      & 1451   \\ \hline
\multirow{4}{*}{6}   & 1    &       & 10   &    \\
    & 2    & 131   & 811  &    \\
    & 3    & 4942  &      & 107    \\
    & 4    &       &      & 1350   \\ \hline
\multirow{4}{*}{7}   & 1    &       & 1    &    \\
    & 2    & 120   & 376  &    \\
    & 3    & 4178  &      & 62     \\
    & 4    &       &      & 1157   \\ \hline
\multirow{3}{*}{8}   & 2    & 82    & 168  &    \\
    & 3    & 3341  &      & 52     \\
    & 4    &       &      & 1032   \\ \hline
\multirow{3}{*}{9}   & 2    & 66    & 51   &    \\
    & 3    & 2498  & 102  & 38     \\
    & 4    &       &      & 836    \\ \hline
\multirow{3}{*}{10}  & 2    & 38    & 22   &    \\
    & 3    & 1897  & 73   & 33     \\
    & 4    &       & 35   & 619    \\ \hline
\end{tabular}
\end{sc}
\end{small}
\end{center}
% \vskip -0.1in
\figspace
\end{table}
